# Supplementary material for: DreamScene: 3D Gaussian-based Text-to-3D Scene Generation via Formation Pattern Sampling
Source: arXiv:2404.03575 source file (2024-07-19)
Supplement: Supplementary file 2 [file supp_bbl.tex]

\begin{thebibliography}{10}
\providecommand{\url}[1]{\texttt{#1}}
\providecommand{\urlprefix}{URL }
\providecommand{\doi}[1]{https://doi.org/#1}

\bibitem{cohen2023set}
Cohen-Bar, D., Richardson, E., Metzer, G., Giryes, R., Cohen-Or, D.: Set-the-scene: Global-local training for generating controllable nerf scenes. arXiv preprint arXiv:2303.13450  (2023)

\bibitem{hollein2023text2room}
H{\"o}llein, L., Cao, A., Owens, A., Johnson, J., Nie{\ss}ner, M.: Text2room: Extracting textured 3d meshes from 2d text-to-image models. arXiv preprint arXiv:2303.11989  (2023)

\bibitem{lin2023componerf}
Lin, Y., Bai, H., Li, S., Lu, H., Lin, X., Xiong, H., Wang, L.: Componerf: Text-guided multi-object compositional nerf with editable 3d scene layout. arXiv preprint arXiv:2303.13843  (2023)

\bibitem{ouyang2023text2immersion}
Ouyang, H., Heal, K., Lombardi, S., Sun, T.: Text2immersion: Generative immersive scene with 3d gaussians. arXiv preprint arXiv:2312.09242  (2023)

\bibitem{rombach2022high}
Rombach, R., Blattmann, A., Lorenz, D., Esser, P., Ommer, B.: High-resolution image synthesis with latent diffusion models. In: Proceedings of the IEEE/CVF conference on computer vision and pattern recognition. pp. 10684--10695 (2022)

\bibitem{vilesov2023cg3d}
Vilesov, A., Chari, P., Kadambi, A.: Cg3d: Compositional generation for text-to-3d via gaussian splatting. arXiv preprint arXiv:2311.17907  (2023)


\bibitem{zhang2024text2nerf}
Zhang, J., Li, X., Wan, Z., Wang, C., Liao, J.: Text2nerf: Text-driven 3d scene generation with neural radiance fields. IEEE Transactions on Visualization and Computer Graphics  (2024)

\bibitem{zhang2023scenewiz3d}
Zhang, Q., Wang, C., Siarohin, A., Zhuang, P., Xu, Y., Yang, C., Lin, D., Zhou, B., Tulyakov, S., Lee, H.Y.: Scenewiz3d: Towards text-guided 3d scene composition. arXiv preprint arXiv:2312.08885  (2023)

\bibitem{zhou2024gala3d}
Zhou, X., Ran, X., Xiong, Y., He, J., Lin, Z., Wang, Y., Sun, D., Yang, M.H.: Gala3d: Towards text-to-3d complex scene generation via layout-guided generative gaussian splatting. arXiv preprint arXiv:2402.07207  (2024)

\end{thebibliography}
